# Supplementary material for: Scaling physics-informed hard constraints with mixture-of-experts
Source: arXiv:2402.13412 source file (2024-02-20)
Supplement: Supplementary file 1 [file appendix-reaction-diffusion.tex]

\longedit
\section{Additional Experiment: 2D Reaction-Diffusion}
\label{subsec:reaction-diffusion}
The 2D reaction-diffusion system describes the interaction between an activator, $u$, and inhibitor, $v$. 
The governing equations model many biological phenomena~\citep{turing_chemical_1990}, including tissue growth.
In contrast to both 1D diffusion-sorption and 2D Navier-Stokes, the learning objective is to learn two time-dependent non-linearly coupled scalar fields ($u$ and $v$), described by:

\begin{align}
    \frac{\partial u (t, x, y)}{\partial t} &= D_u \frac{\partial^2 u(t, x, y)}{\partial x^2} + D_u \frac{\partial ^ 2 u(t, x, y)}{\partial y^2} + R_u, & x, y \in (0, 1), t \in (0, 5] \\
    \frac{\partial v(t, x, y)}{\partial t} &= D_v \frac{\partial^2 v(t, x, y)}{\partial x^2 } + D_u \frac{\partial^2 v(t, x, y)}{\partial y^2} + R_v,
\end{align}

where $R_u$ and $R_v$ are the Fitzhugh-Nagumo equations~\citep{klaasen_stationary_1984}: 

\begin{align}
    R_u(u, v) &= u - u^3 - k - v \\
    R_v(u, v) &= u - v
\end{align}

$D_u=1e^{-3}$, $D_v=5e^{-3}$, and $k=5e^{-3}$ are physical values representing the activator diffusion, inhibitor diffusion, and recovery variable constants. 
For this problem, we use no-flow Neumann boundary conditions.

\paragraph{Problem setup.} Each solution trajectory is solved over $T=5$ seconds, where the initial conditions are draw from a 2D Gaussian random field with a length scale of 5.
The train and test sets contain 800 and 100 unique initial conditions, respectively. 
We use a discretization of 32 ($t$) $\times$ 64 ($x$) $\times$ 64 ($y$). 
To generate numerical solutions, we use PDEBench, which is based on a standard time integrator from SciPy~\citep{virtanen_scipy_2020}. 
PI-SC, PI-HC, and~\hcmoe employ a FNO base architecture with 5 layers, 8 modes, and a hidden dimension size of 64. 
PI-HC and~\hcmoe both use 64 basis functions.
~\hcmoe uses $K=2$ spatial experts along the $y$ dimension.
Each expert and PI-HC sample $10$k points.
We use a learning rate of $1e^{-3}$ with an exponential decay over 50 epochs with early stopping.
The tolerance of the Levenberg-Marquardt solver is set to $1e^{-4}$.

\paragraph{Results.}\fref{fig:err-reaction-diffusion} plots the relative $L_2$ error on the held out validation set over training, and the distribution of errors of each trained model.
PI-SC ($\mathbf{96.876\%\pm0.088\%}$) is unable to converge to a reasonable solution, collapsing to a constant function. 
PI-HC ($\mathbf{29.031\%\pm4.418\%}$) and~\hcmoe ($\mathbf{23.940\%\pm3.074\%}$) both achieve significantly lower error.
Representative examples of both the activator and inhibitor are plotted in Figs.~\ref{fig:rd-0} and~\ref{fig:rd-10} for $t=0$ (s) and $t=1.5625$ (s).
%On later time steps, the solution quality of both PI-HC and~\hcmoe degrade, varying significantly from the numerical solver solution.
%We hypothesize that the physical non-linear least squares constraint may be insufficiently constrained for latter time steps, but formulating a new constraint is left for future work.

\begin{figure}[!htbp]
    \centering
    \includegraphics[width=\textwidth]{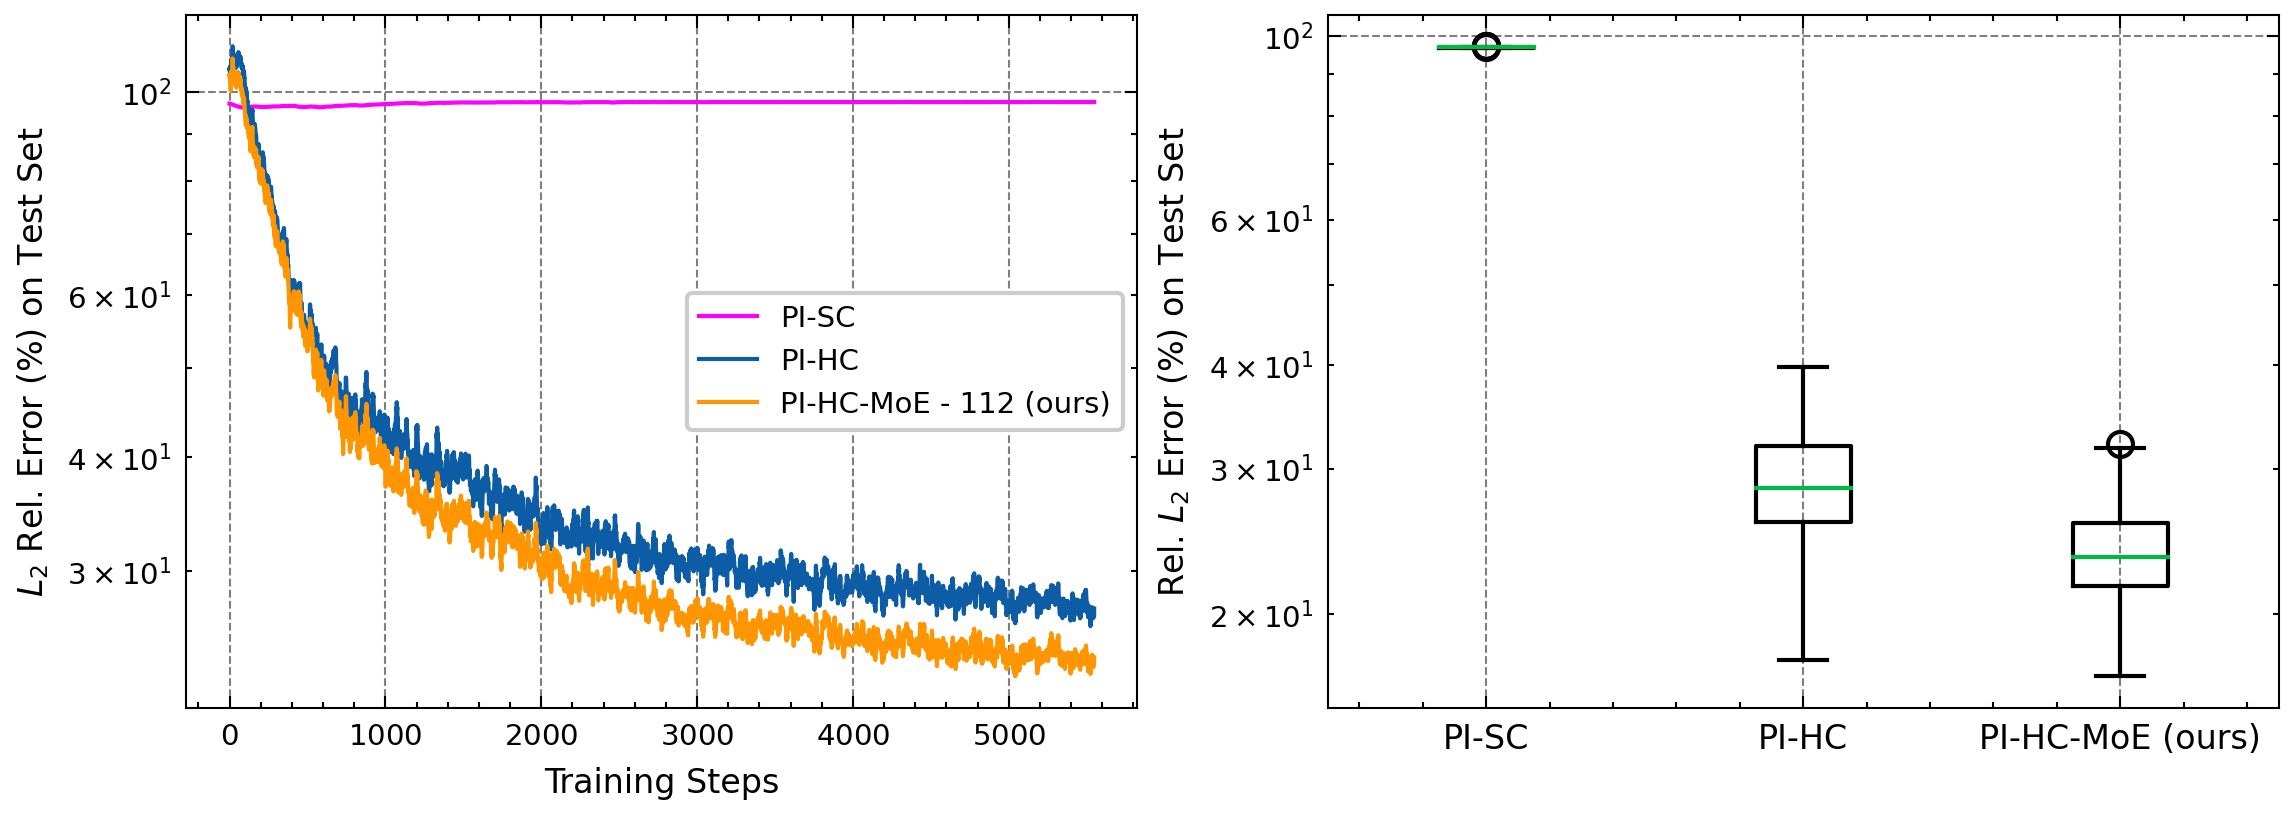}
    \caption{\edit{\textbf{Relative test $L_2$ error on 2D reaction-diffusion}. (Left) Relative $L_2$ over training iterations. (Right) Final distribution of test set errors from the trained models.}}
    \label{fig:err-reaction-diffusion}
\end{figure}

\begin{figure}[!htbp]
    \centering
    \includegraphics[width=\textwidth]{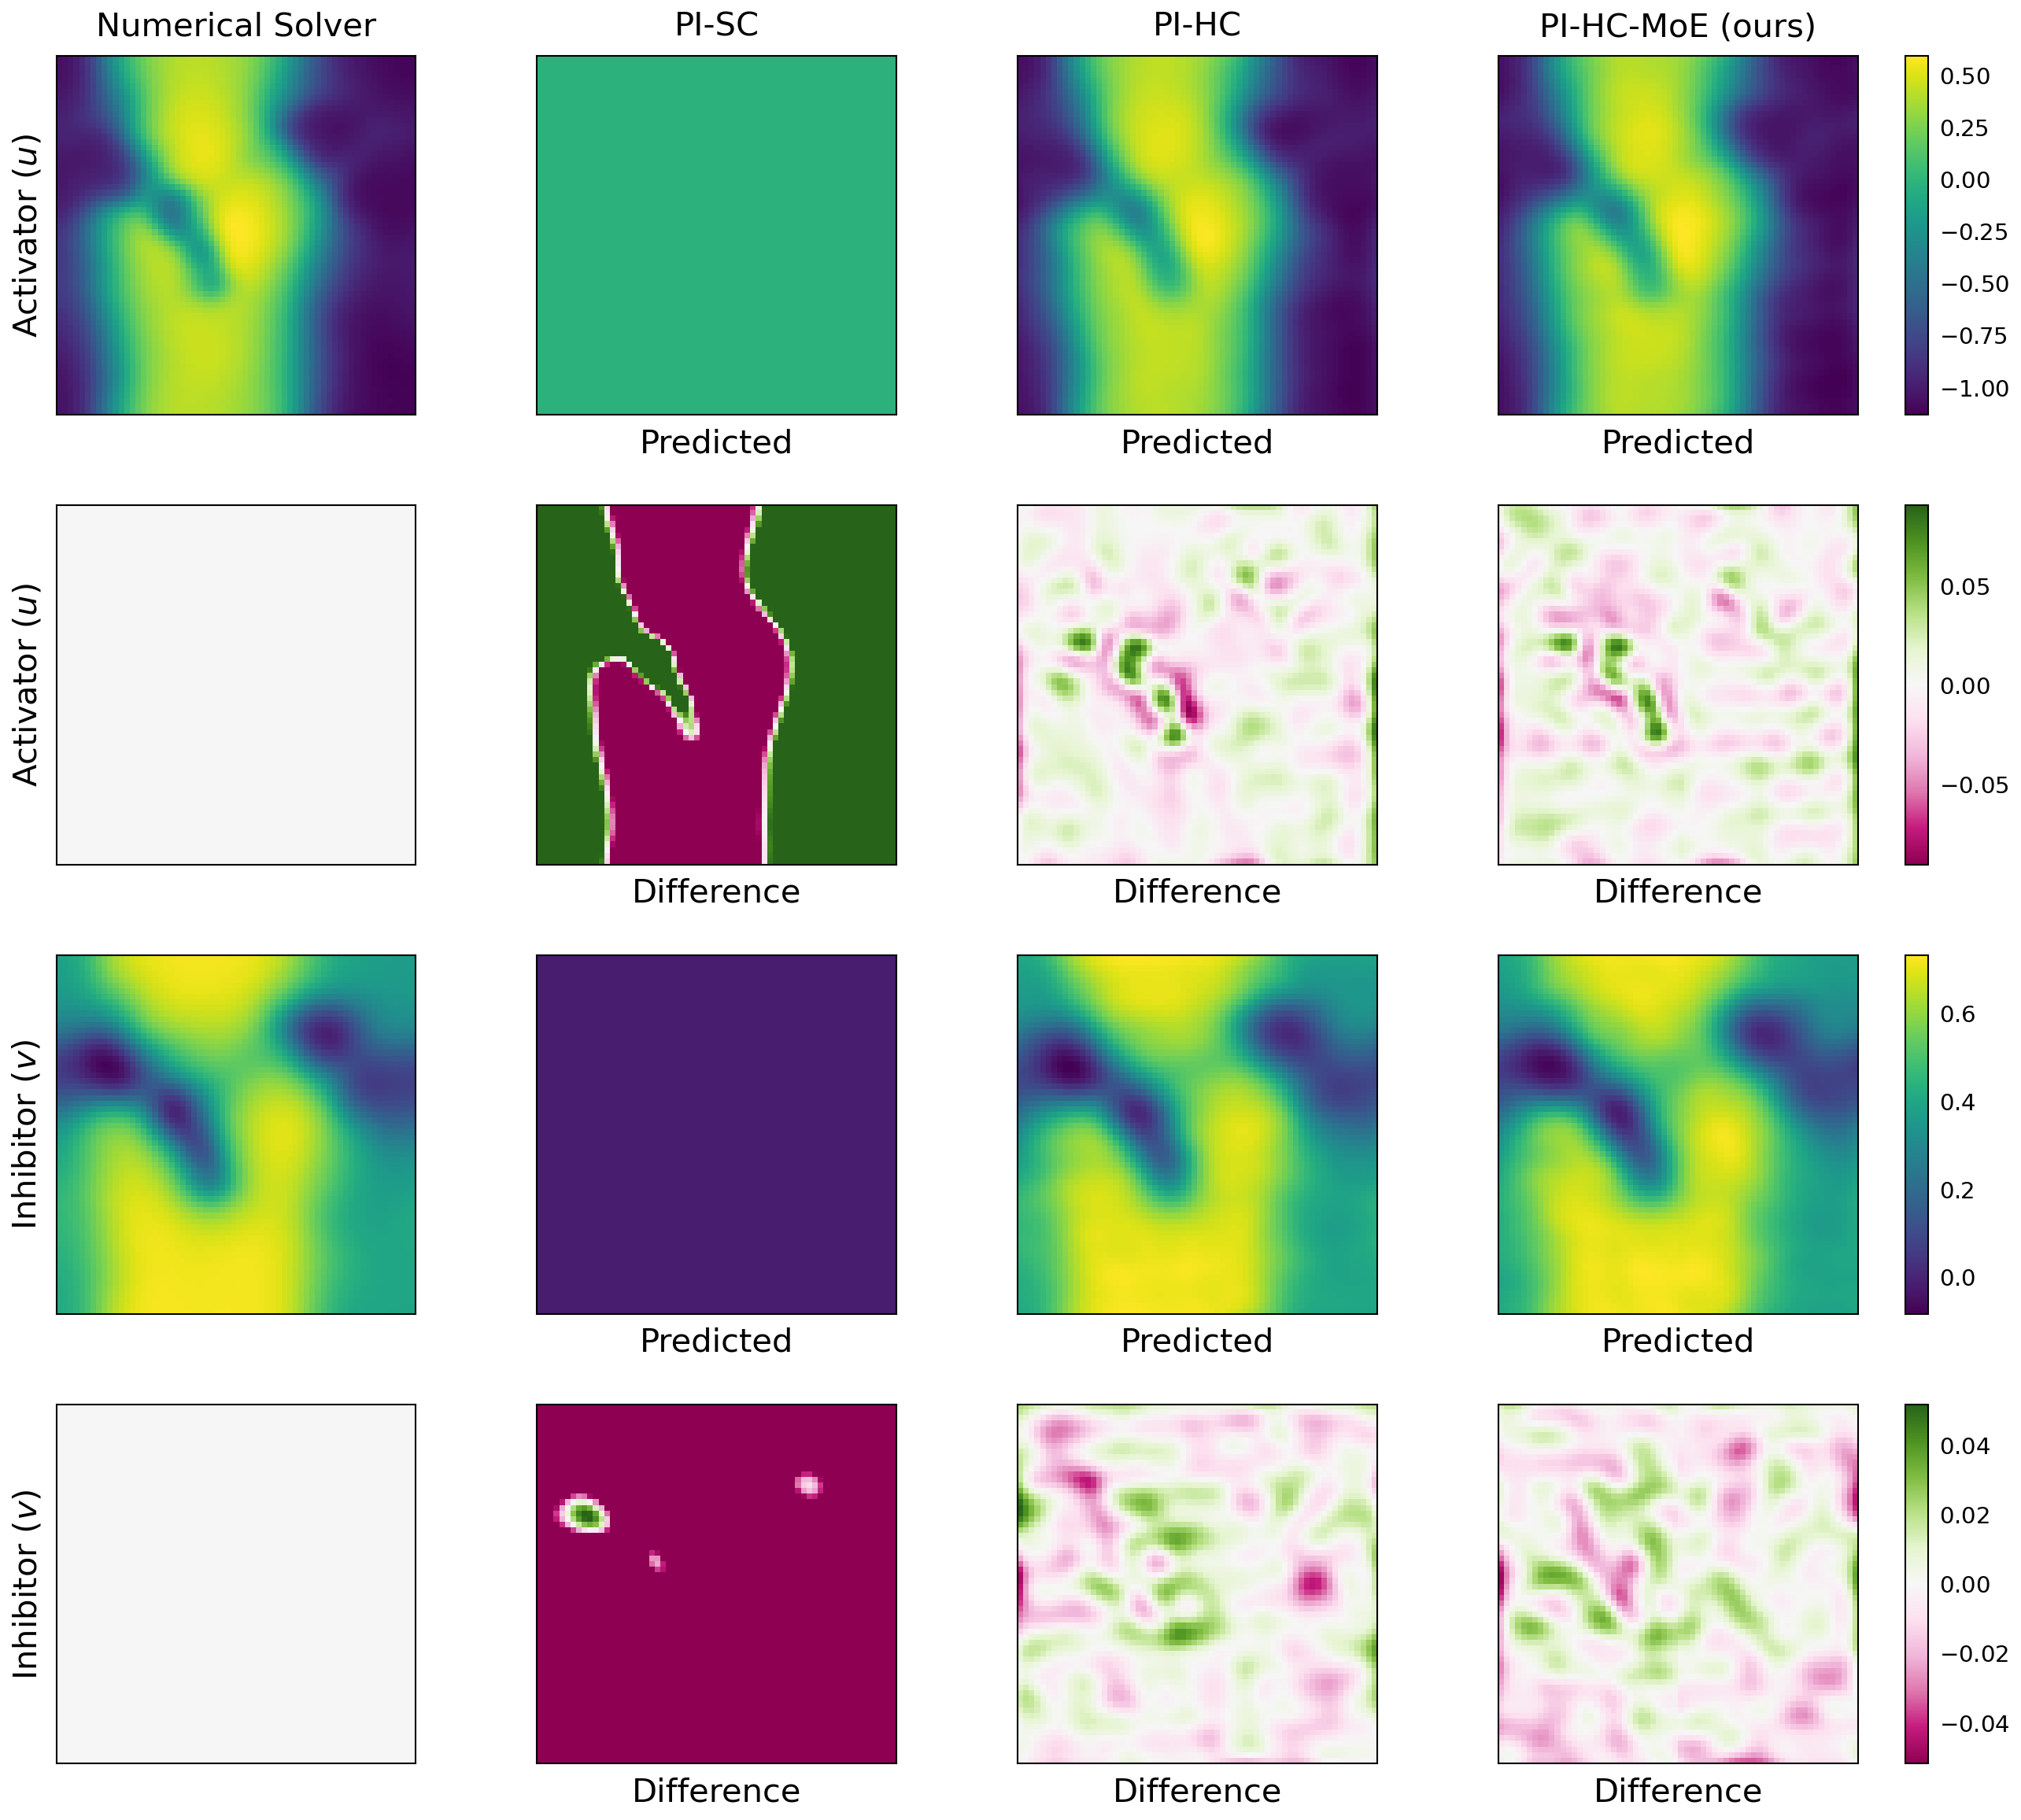}
    \caption{\edit{\textbf{Predicted solution at $t=0$ (s)  of 2D reaction-diffusion.} From top to bottom: (Row 1) Predicted activator $u$. (Row 2) Difference between the predicted activator and numerical solver solution. PI-SC differences are clipped to the colorbar. (Row 3) Predicted inhibitor $v$. (Row 4) Difference between the predicted inhibitor and numerical solver solution. PI-SC differences are clipped to the colorbar.}}
    \label{fig:rd-0}
\end{figure}

\begin{figure}[!htbp]
    \centering
    \includegraphics[width=\textwidth]{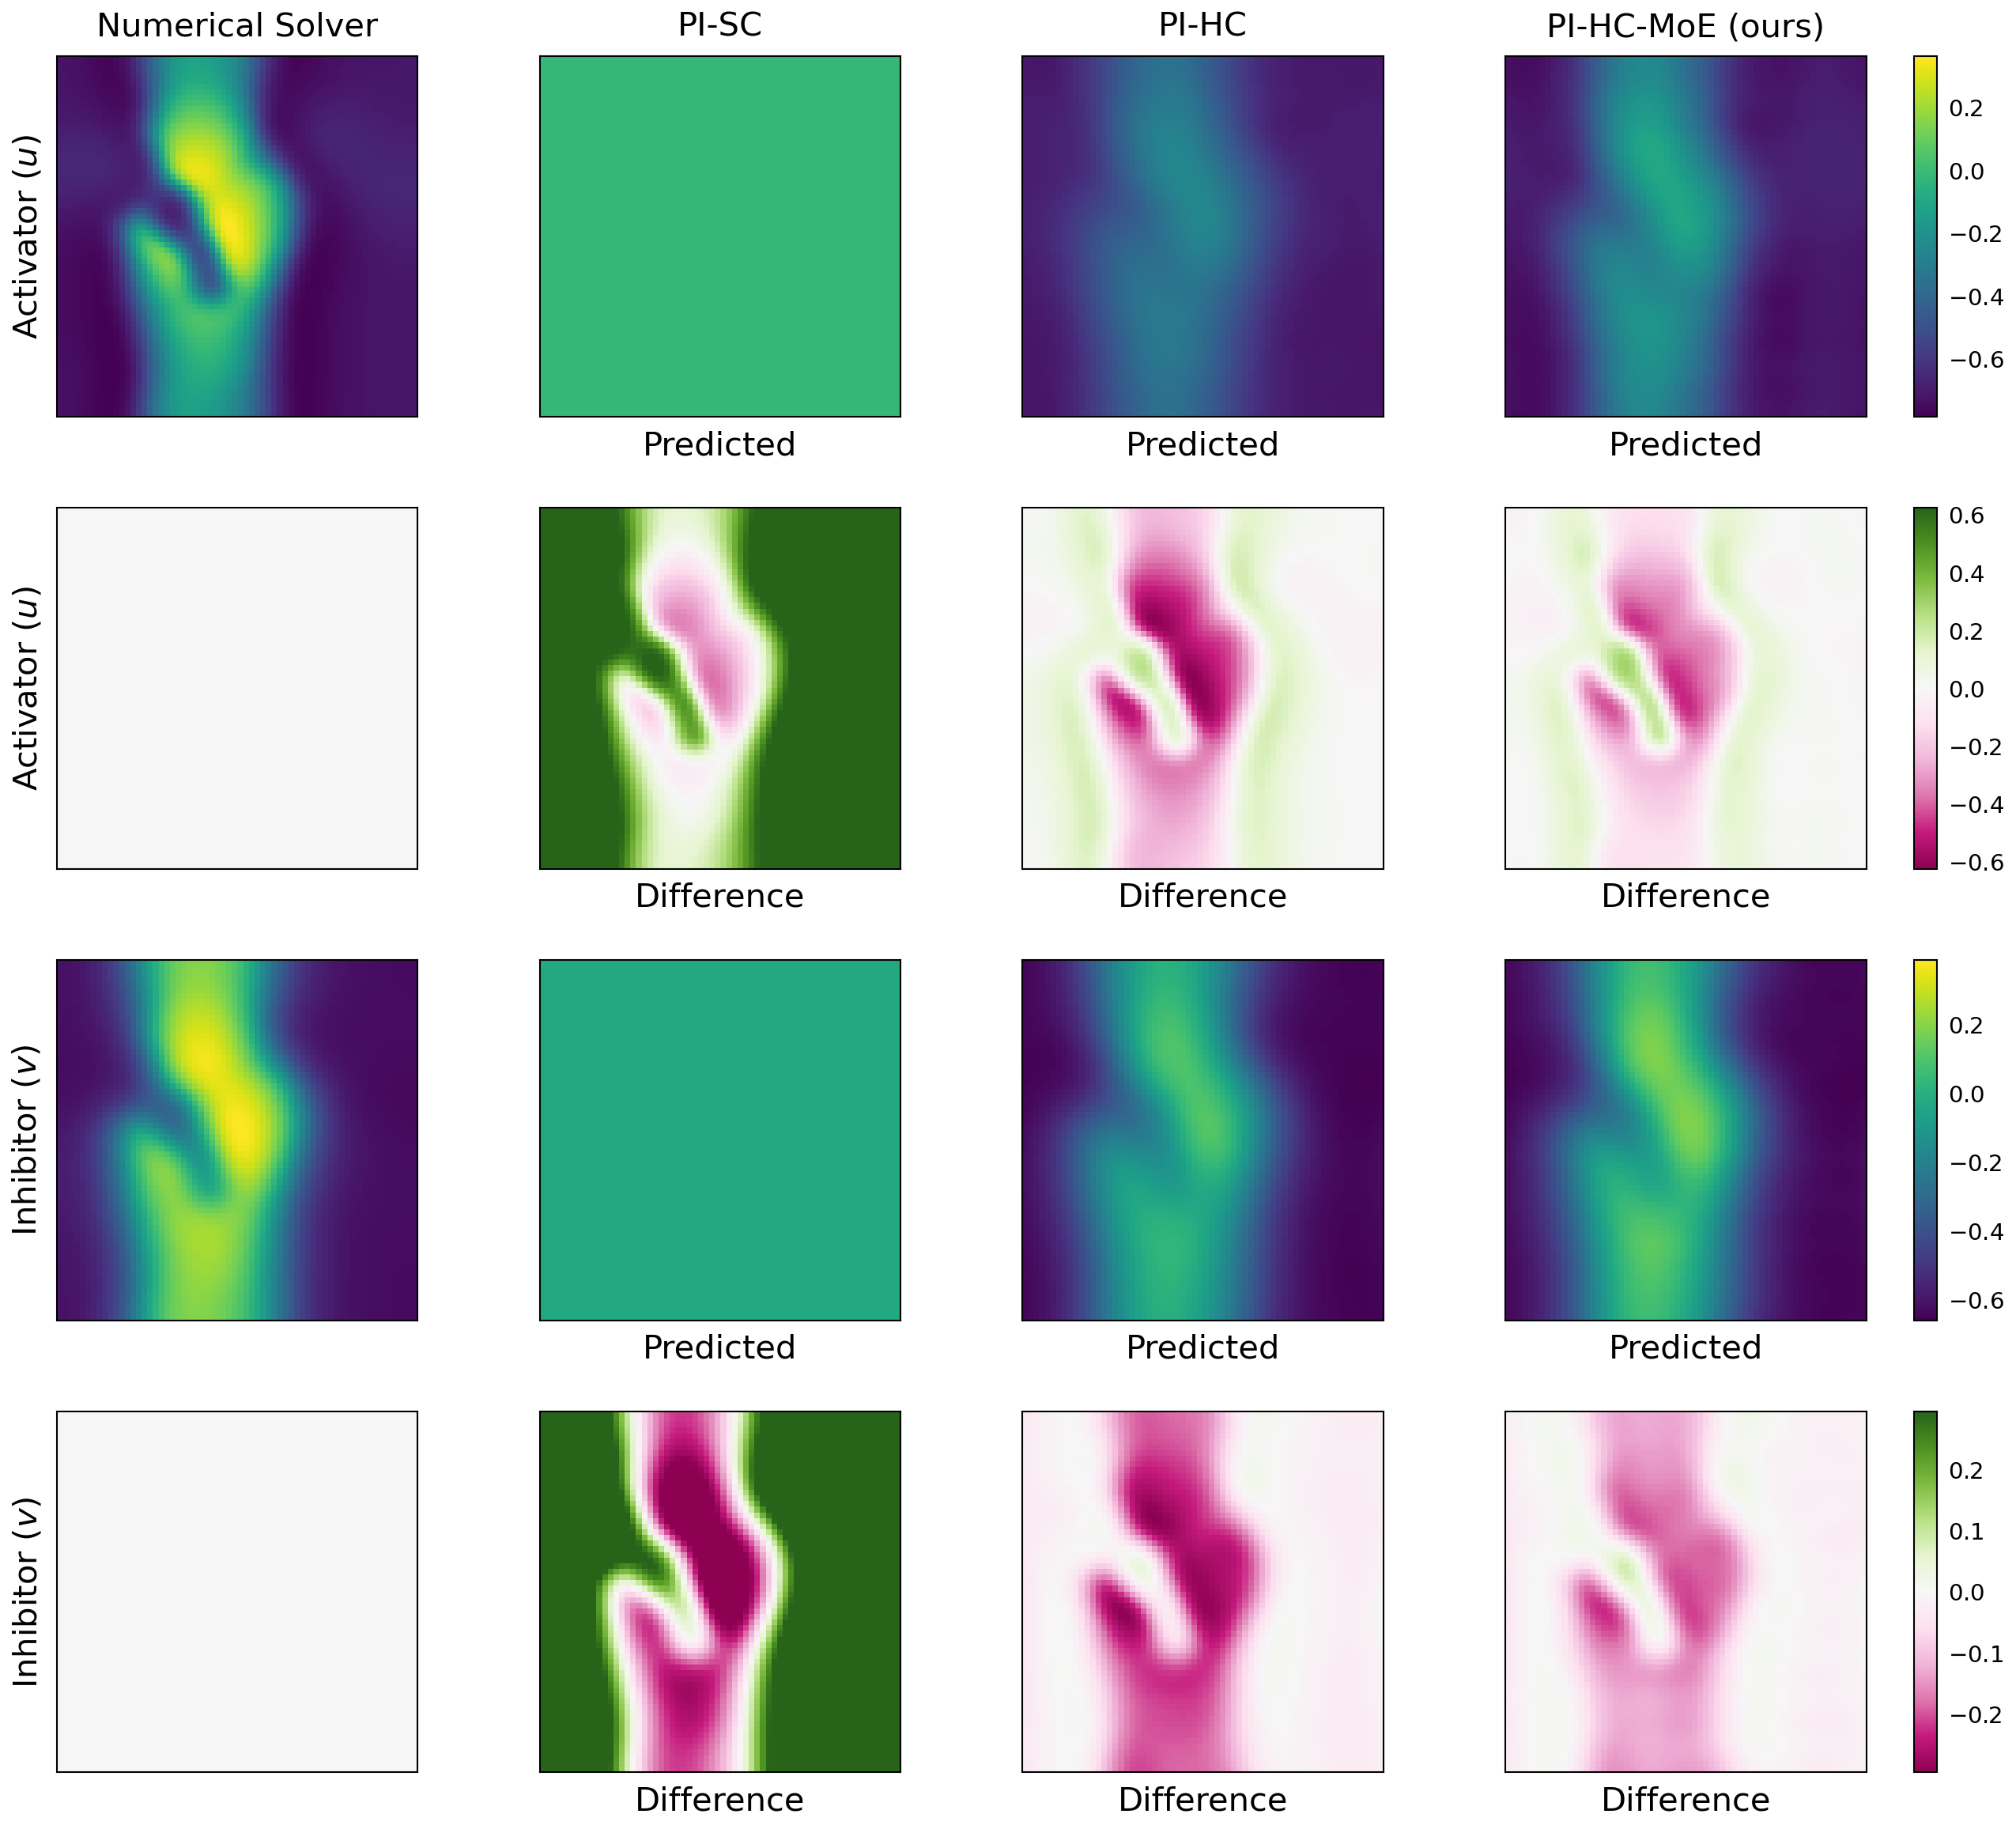}
    \caption{\edit{\textbf{Predicted solution at $t=1.5625$ (s)  of 2D reaction-diffusion.} From top to bottom: (Row 1) Predicted activator $u$. (Row 2) Difference between the predicted activator and numerical solver solution. PI-SC differences are clipped to the colorbar. (Row 3) Predicted inhibitor $v$. (Row 4) Difference between the predicted inhibitor and numerical solver solution. PI-SC differences are clipped to the colorbar.}}
    \label{fig:rd-10}
\end{figure}

\longeditend
