# Supplementary material for: Scaling physics-informed hard constraints with mixture-of-experts
Source: arXiv:2402.13412 source file (2024-02-20)
Supplement: Supplementary file 2 [file appendix-diffusion-sorption-alias.tex]

\longedit
\section{Additional Diffusion-Sorption Prediction Visualizations}

In~\fref{fig:ds-heatmaps},~\hcmoe exhibits some grid-like artifacts.
To investigate whether these artifacts are systemic, we randomly sample 16 different predicted instances which are plotted in~\fref{fig:ds-alias-predictions}.
To the best of our knowledge, this is not a common occurrence, and none of the sampled 16 instances have any noticeable artifacts.

\begin{figure}[!htbp]
    \centering
    \includegraphics[width=\textwidth]{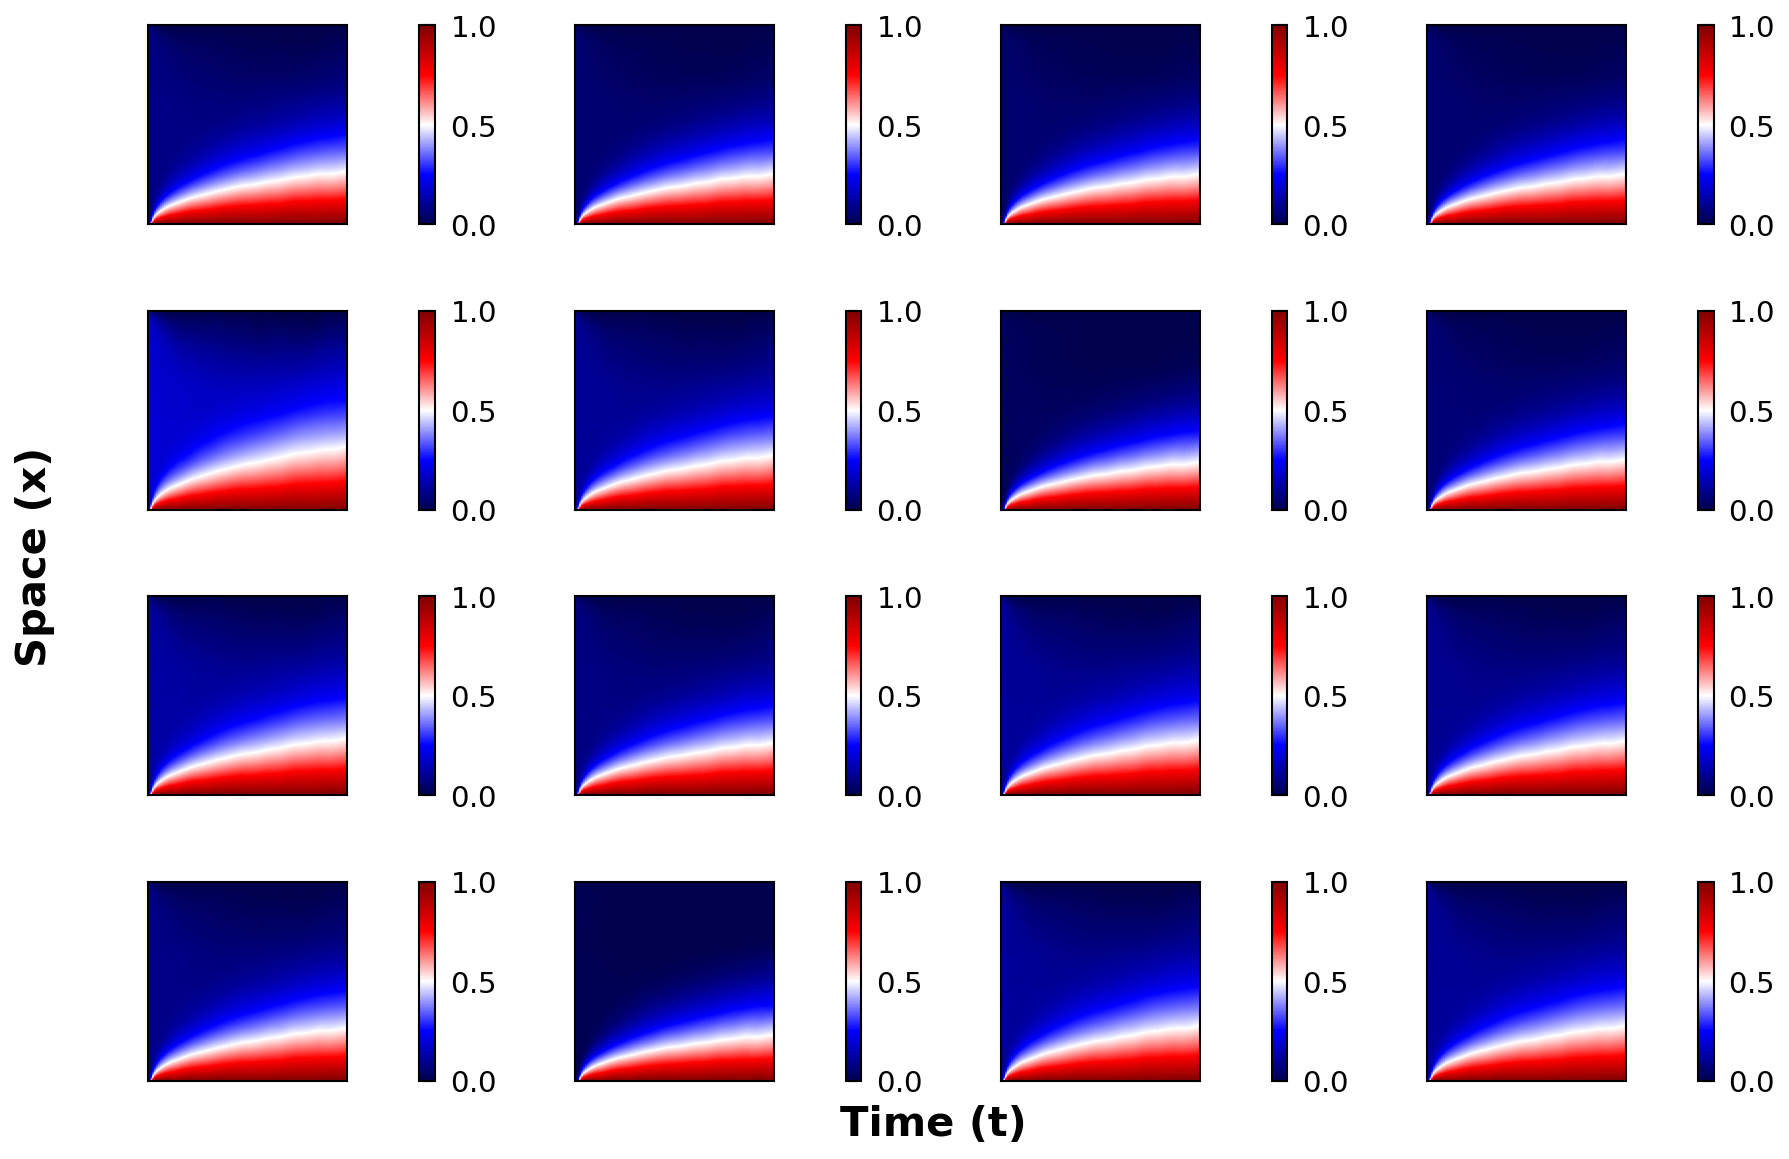}
    \caption{\edit{\textbf{16 randomly sampled predictions by~\hcmoe for diffusion-sorption.}}}
    \label{fig:ds-alias-predictions}
\end{figure}

\longeditend
