# Supplementary material for: Scaling physics-informed hard constraints with mixture-of-experts
Source: arXiv:2402.13412 source file (2024-02-20)
Supplement: Supplementary file 3 [file appendix-notation.tex]

% \section{Math Notation}

% List of Symbols used: \ak{Could potentially make this a table at the top of the page (and/or move it to appendix)}
% \begin{enumerate}
%     \item NN $\mathcal{G_\theta}: \phi \rightarrow u_\theta$
%     \item Opt func $\mathcal{F}_\phi(u)=\mathbf{0}$
%     \item Basis functions $f_\theta: \phi \rightarrow \mathbf{b}$. Basis function indexing $f^i$, $N$ number of basis functions
%     \item $m$ sampled points
%     \item $G$ represents a non-linear least squares solver
%     \item $K$ Number of experts
%     \item $\Omega_k$ the domain of expert $k$
%     \item $\Omega$ defines the spatial-temporal grid
% \end{enumerate}

% \begin{table}[h]
% \centering
% \begin{tabular}{|l|l|}
% \hline
% \textbf{Symbol}                   & \textbf{Meaning}                                                              \\ \hline
% $\Omega$                          & Domain of the PDE                                                             \\ \hline
% $\mathcal{F}_\phi$                & PDE  equations parameterized by $\phi$                                        \\ \hline
% $u$                               & The solution to a PDE                                                         \\ \hline
% $\mathcal{G}_\theta$              & A neural operator parameterized by $\theta$ mapping from $\phi$ to $u_\theta$ \\ \hline
% $u_\theta$                        & The predicted solution to a PDE                                               \\ \hline
% $\mathbf{b} = [f^0, f^1 ... f^N]$ & Basis functions predicted by $f_\theta$                                       \\ \hline
% $N$                               & The number of basis functions                                                 \\ \hline
% $m$                               & The number of sampled points                                                  \\ \hline
% $G$                               & The nonlinear least squares solver                                            \\ \hline
% $\omega$                          & The weighting of basis functions                                              \\ \hline
% $K$                               & The number of experts                                                         \\ \hline
% $\Omega_k$                        & The domain of expert $k$                                                      \\ \hline
% \end{tabular}
% \end{table}
